# Supplementary material for: Object Placement Planning and Optimization for Robot Manipulators
Source: arXiv:1907.02555 source file (2019-07-04)
Supplement: Supplementary file 1 [file appendix.tex]

\appendix
\subsection{Error Functions and Collision cost}
The error functions $e_\xi, e_{\hat{S}}, e_{c_f}, e_\sigma: \mathcal{C}_o \to \mathbb{R}^{\geq 0}$,
as well as the arm collision cost $c: \mathcal{C}_r \to \mathbb{R}^{\geq 0}$ map their arguments
to values greater $0$, if their argument violates their respective constraint, and to $0$ otherwise.
We present the definition of each of these functions in the following
subsections. Conceptually, all of these functions
are similar to obstacle cost functions applied in works on trajectory optimization~\cite{Zucker2013, Mukadam2016}.
All functions depend on some task space distance functions $d_i:\textit{SE}(3) \to \mathbb{R}$
that map the position or rotation angle from a pose onto a distance to, e.g. a collision-free
position, a position within a placement contact region, or to some range of values.
To render these distances smooth, we adopt the following function from \cite{Zucker2013}:
\begin{equation}
        \delta(d_i(\bm{p})) = \begin{cases}
                -d_i(\bm{p}) + \frac{\epsilon_i}{2}             &\mbox{if } d_i(\bm{p}) < 0 \\
                \frac{1}{2\epsilon_i}(d_i(\bm{p}) - \epsilon_i)^2  &\mbox{if } 0 \leq d_i(\bm{p}) \leq \epsilon_i \\
                0                                           &\mbox{else}
                \end{cases}
        \label{eq:delta_err}
\end{equation}
with some constant $\epsilon_i \in \mathbb{R}^{\geq 0}$.

\subsubsection{Objective error $e_\xi$}
The purpose of the objective error $e_\xi$ is to guide \algref{algo:projection} towards
configurations that reach an object pose $\bm{p} \in \mathcal{C}_o$ with objective value
$\xi(\bm{p}) > \xi_\text{best}$, where $\xi_\text{best}$ is the best objective value a solution
is known for so far. For this purpose, we define the error function on the object pose as:
\begin{equation}
  e_\xi(\bm{p}) = \delta(\xi(\bm{p}) - \xi_\text{best})
\end{equation}
To compute the gradient of $\frac{\partial e_\xi(\bm{p})}{\partial x, y, e_z}$, we compute
the gradient $\frac{\partial \xi(\bm{p})}{\partial x, y, e_z}$ numerically.

\subsubsection{In-region error $e_{\hat{S}}$}
The error function $e_{\hat{S}}$ is designed to guide \algref{algo:projection} towards
poses that achieve contact, as well as to force it to reach different subsets
of $\hat{S}(r, f) = \hat{S}(r, f, 0, 2\pi)$. For $\hat{S}(r, f, \check{\theta}, \hat{\theta})$,
the error function is defined as:
\begin{equation}
        e_{\hat{S}}(\bm{p}) = \delta(d_r(\bm{p})) + \delta(d_\theta(\bm{p}))
\end{equation}
with
\begin{equation}
        d_{r}(\bm{p}) = -\underset{(x, y, z)^T \in r}{\min}\| \begin{pmatrix}x \\ y \\ z\end{pmatrix}
                - \begin{pmatrix}p_x \\ p_y \\ p_z\end{pmatrix} \| + \epsilon_r
\end{equation}
and
\begin{equation}
        d_{\theta}(\bm{p}) = -\max(\check{\theta} - p_{e_z}, p_{e_z} - \hat{\theta}) + \epsilon_\theta
\end{equation}

\subsubsection{Stability error $e_{\sigma}$}
For a pose $\bm{p} \in \mathcal{C}_o$ to be actually stable, all vertices of the placement face
must be in contact with placement regions. Hence, we define the stability error:
\begin{equation}
        e_{\sigma}(\bm{p}) = \sum_{\bm{p'} \in v(f, \bm{p})} \delta(d_{r}(p')),
\end{equation}
where $\bm{p'} \in v(f, \bm{p})$ are the poses arising from translating $\bm{p}$ by
the relative positions of the vertices of the placement face.

\subsubsection{Collision error $e_{c_f}$}
The collision error is designed to guide \algref{algo:projection} towards collision-free,
that is physically feasible, placement poses. It is defined as
\begin{equation}
        e_{c_f}(\bm{p}) = \sum_{p' \in \mathcal{B}_o(\bm{p})} \delta(d_{\mathcal{S}}(\bm{p'})),
\end{equation}
where $\mathcal{B}_o(\bm{p})$ denotes a set of positions that approximate the volume
of the object $o$ covered if it is located in pose $\bm{p}$.
The distance function $d_{\mathcal{S}}: \mathbb{R}^3 \to \mathbb{R}$
in this case is the signed distance to the environments surface.

\subsubsection{Arm collision cost $c$}
In contrast, to the above collision cost, the arm collision cost $c$ is designed to
guide \algref{algo:projection} towards collision-free arm configurations. It is defined as
\begin{equation}
        c(q) = \sum_{(p_i, r_i) \in \mathcal{B}_r(q)} \delta(d_{\mathcal{S}}(p_i) - r_i).
\end{equation}
Similar to \cite{Zucker2013}, we approximate the robot by a set of balls
$\mathcal{B}_r = \{(p_i, r_i)\}_{i=1}^b$ to compute this cost efficiently.
